# Supplementary material for: Balanced Multi-modal Federated Learning via Cross-Modal Infiltration
Source: arXiv:2401.00894 source file (2023-12-31)
Supplement: Supplementary file 1 [file X_suppl.tex]

\clearpage
\setcounter{page}{1}
\maketitlesupplementary

\section{Reproducibility}
\subsection{Computing Infrastructure}
All of our experiments were conducted on one NVIDIA GeForce RTX 3090 GPU. Python version: 3.9. CUDA Version: 11.7.

\subsection{Data Division}
We use Dirichlet distribution for non-IID data partition. $\alpha =5$ for CREMA-D and $\alpha =3$ for AVE. We demonstrate the detailed sample size on CREMA-D as shown in \cref{fig:CREMAD client sample}. It's clear that the total sample number of each client varies and the class-wise sample distributions are also different among clients. Similar results can be found in AVE and CrisisMMD.

\begin{figure}[h]
    \centering
    \begin{subfigure}{0.49\linewidth}
        \includegraphics[width=1.0\linewidth]{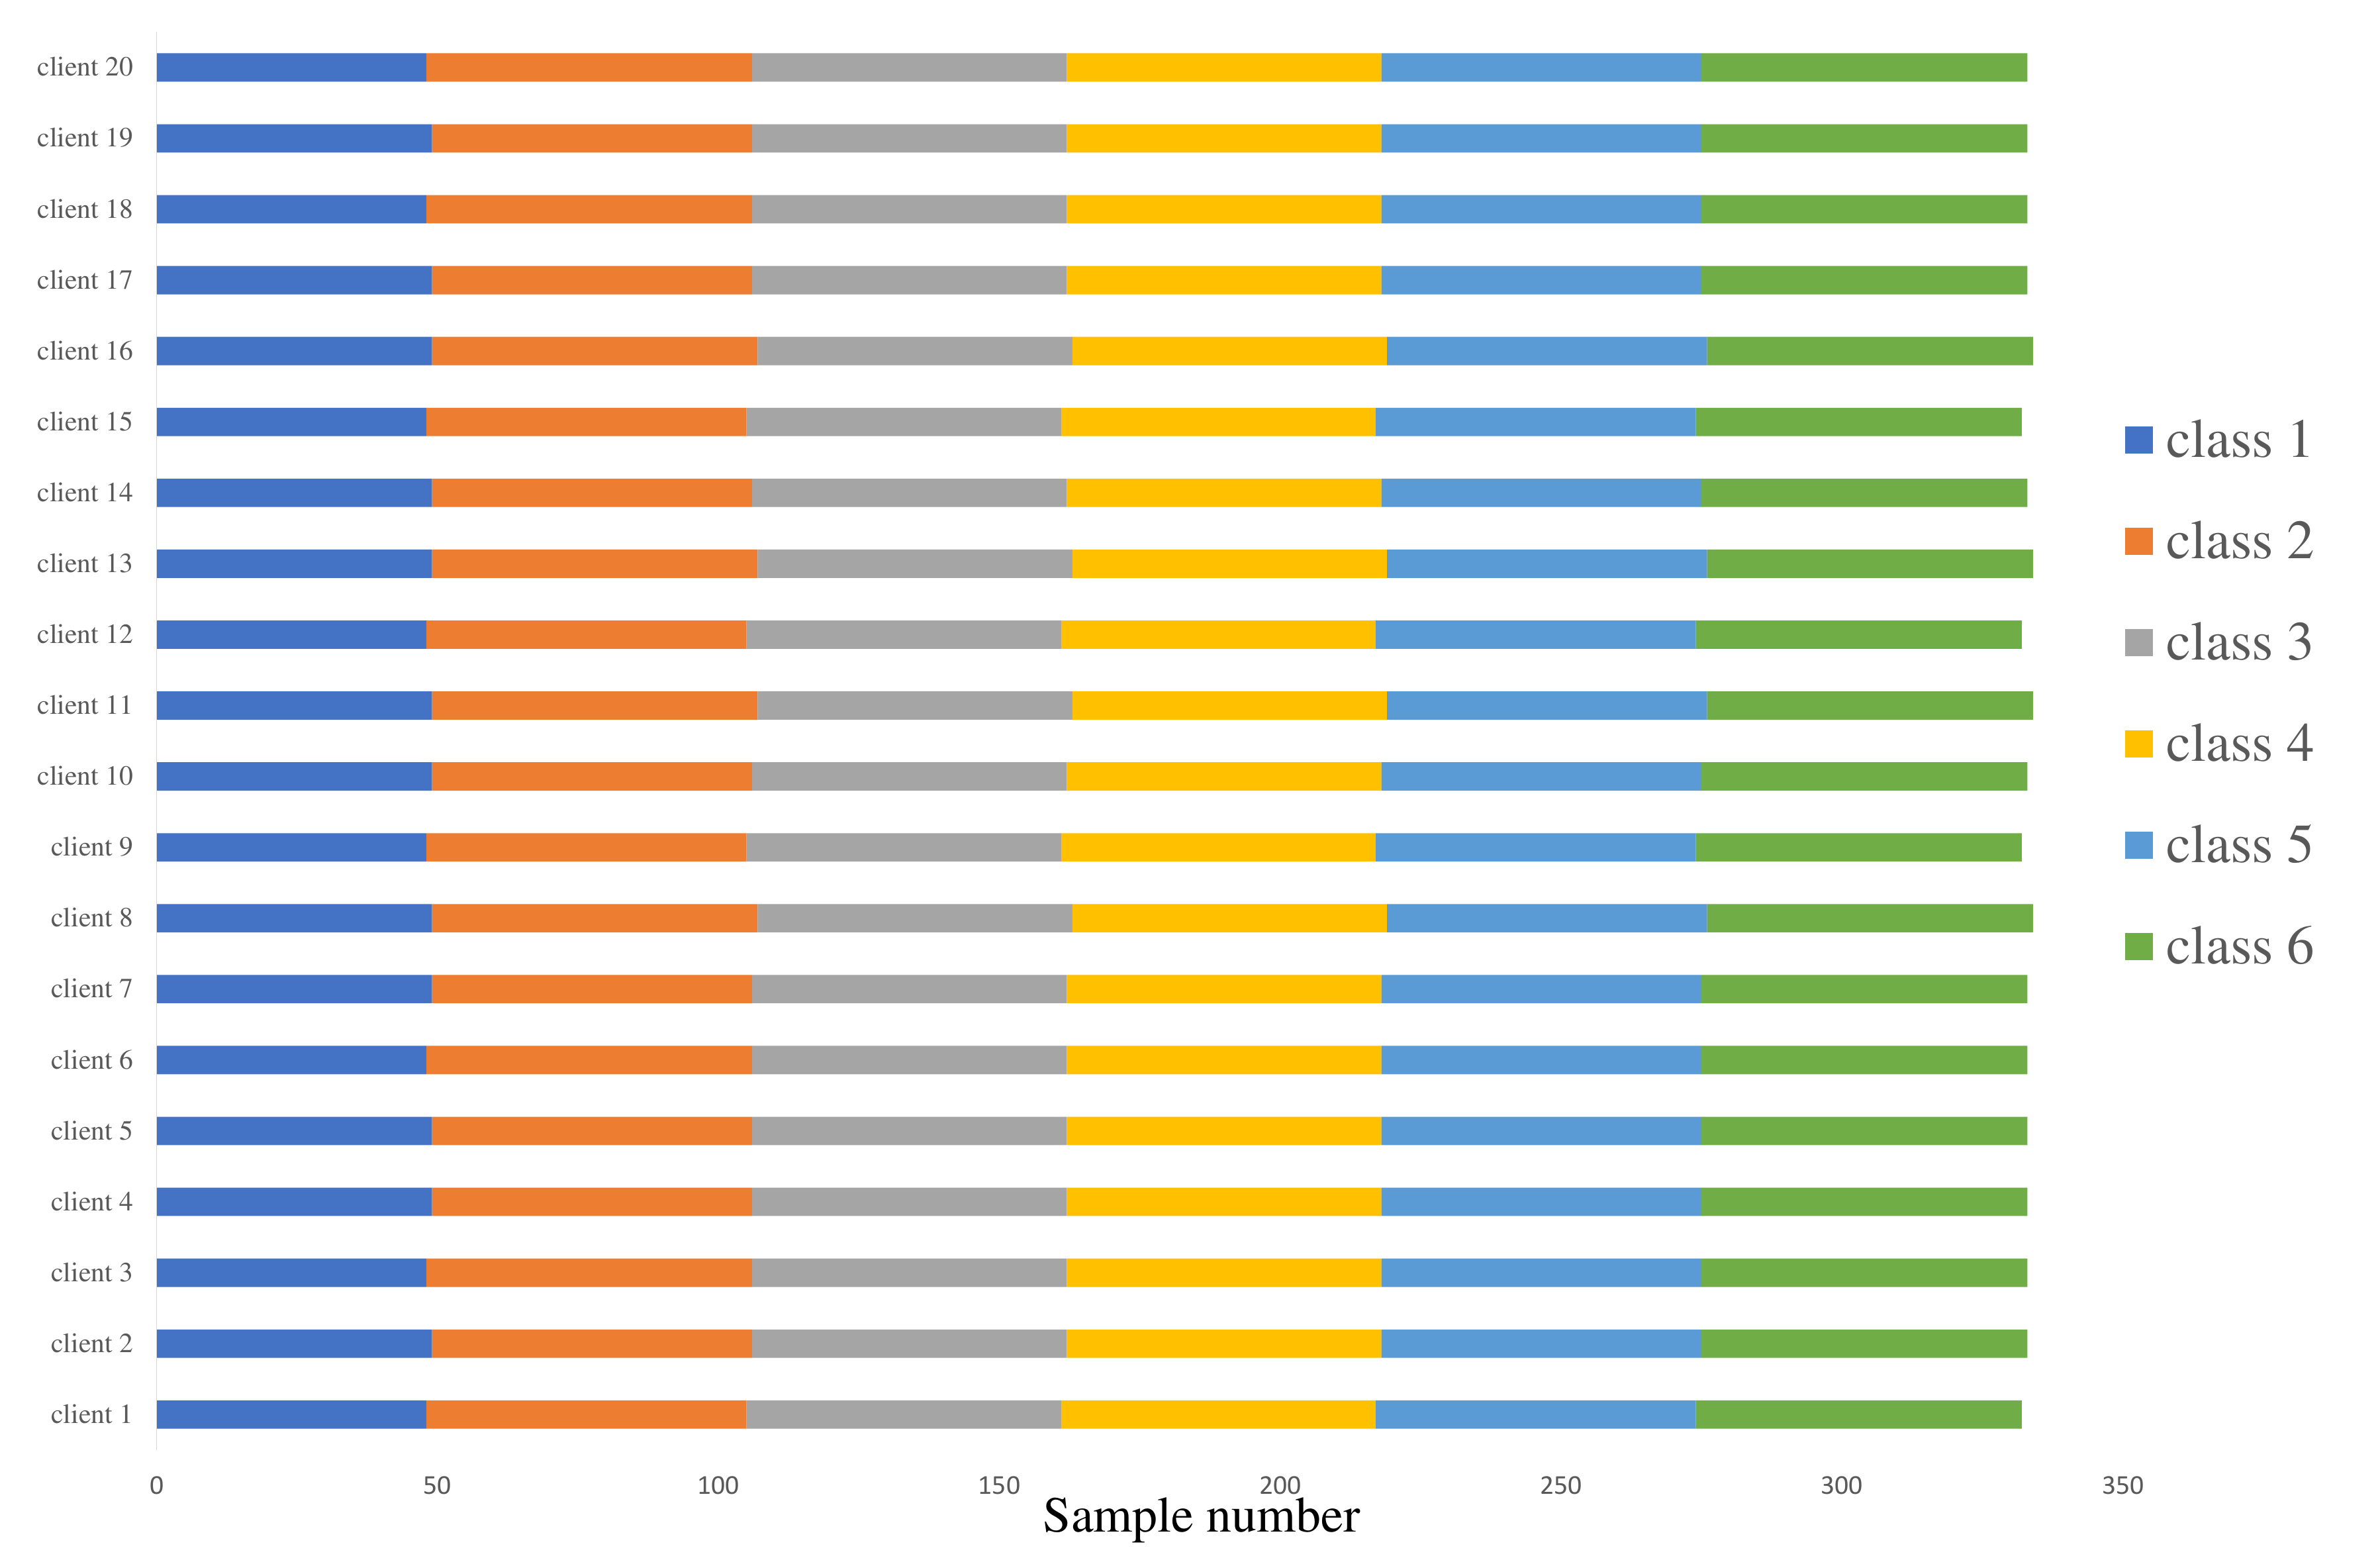}
        \caption{IID}
        \label{fig:audio acc AVE}
    \end{subfigure}
    \hfill
    \begin{subfigure}{0.49\linewidth}
        \includegraphics[width=1.0\linewidth]{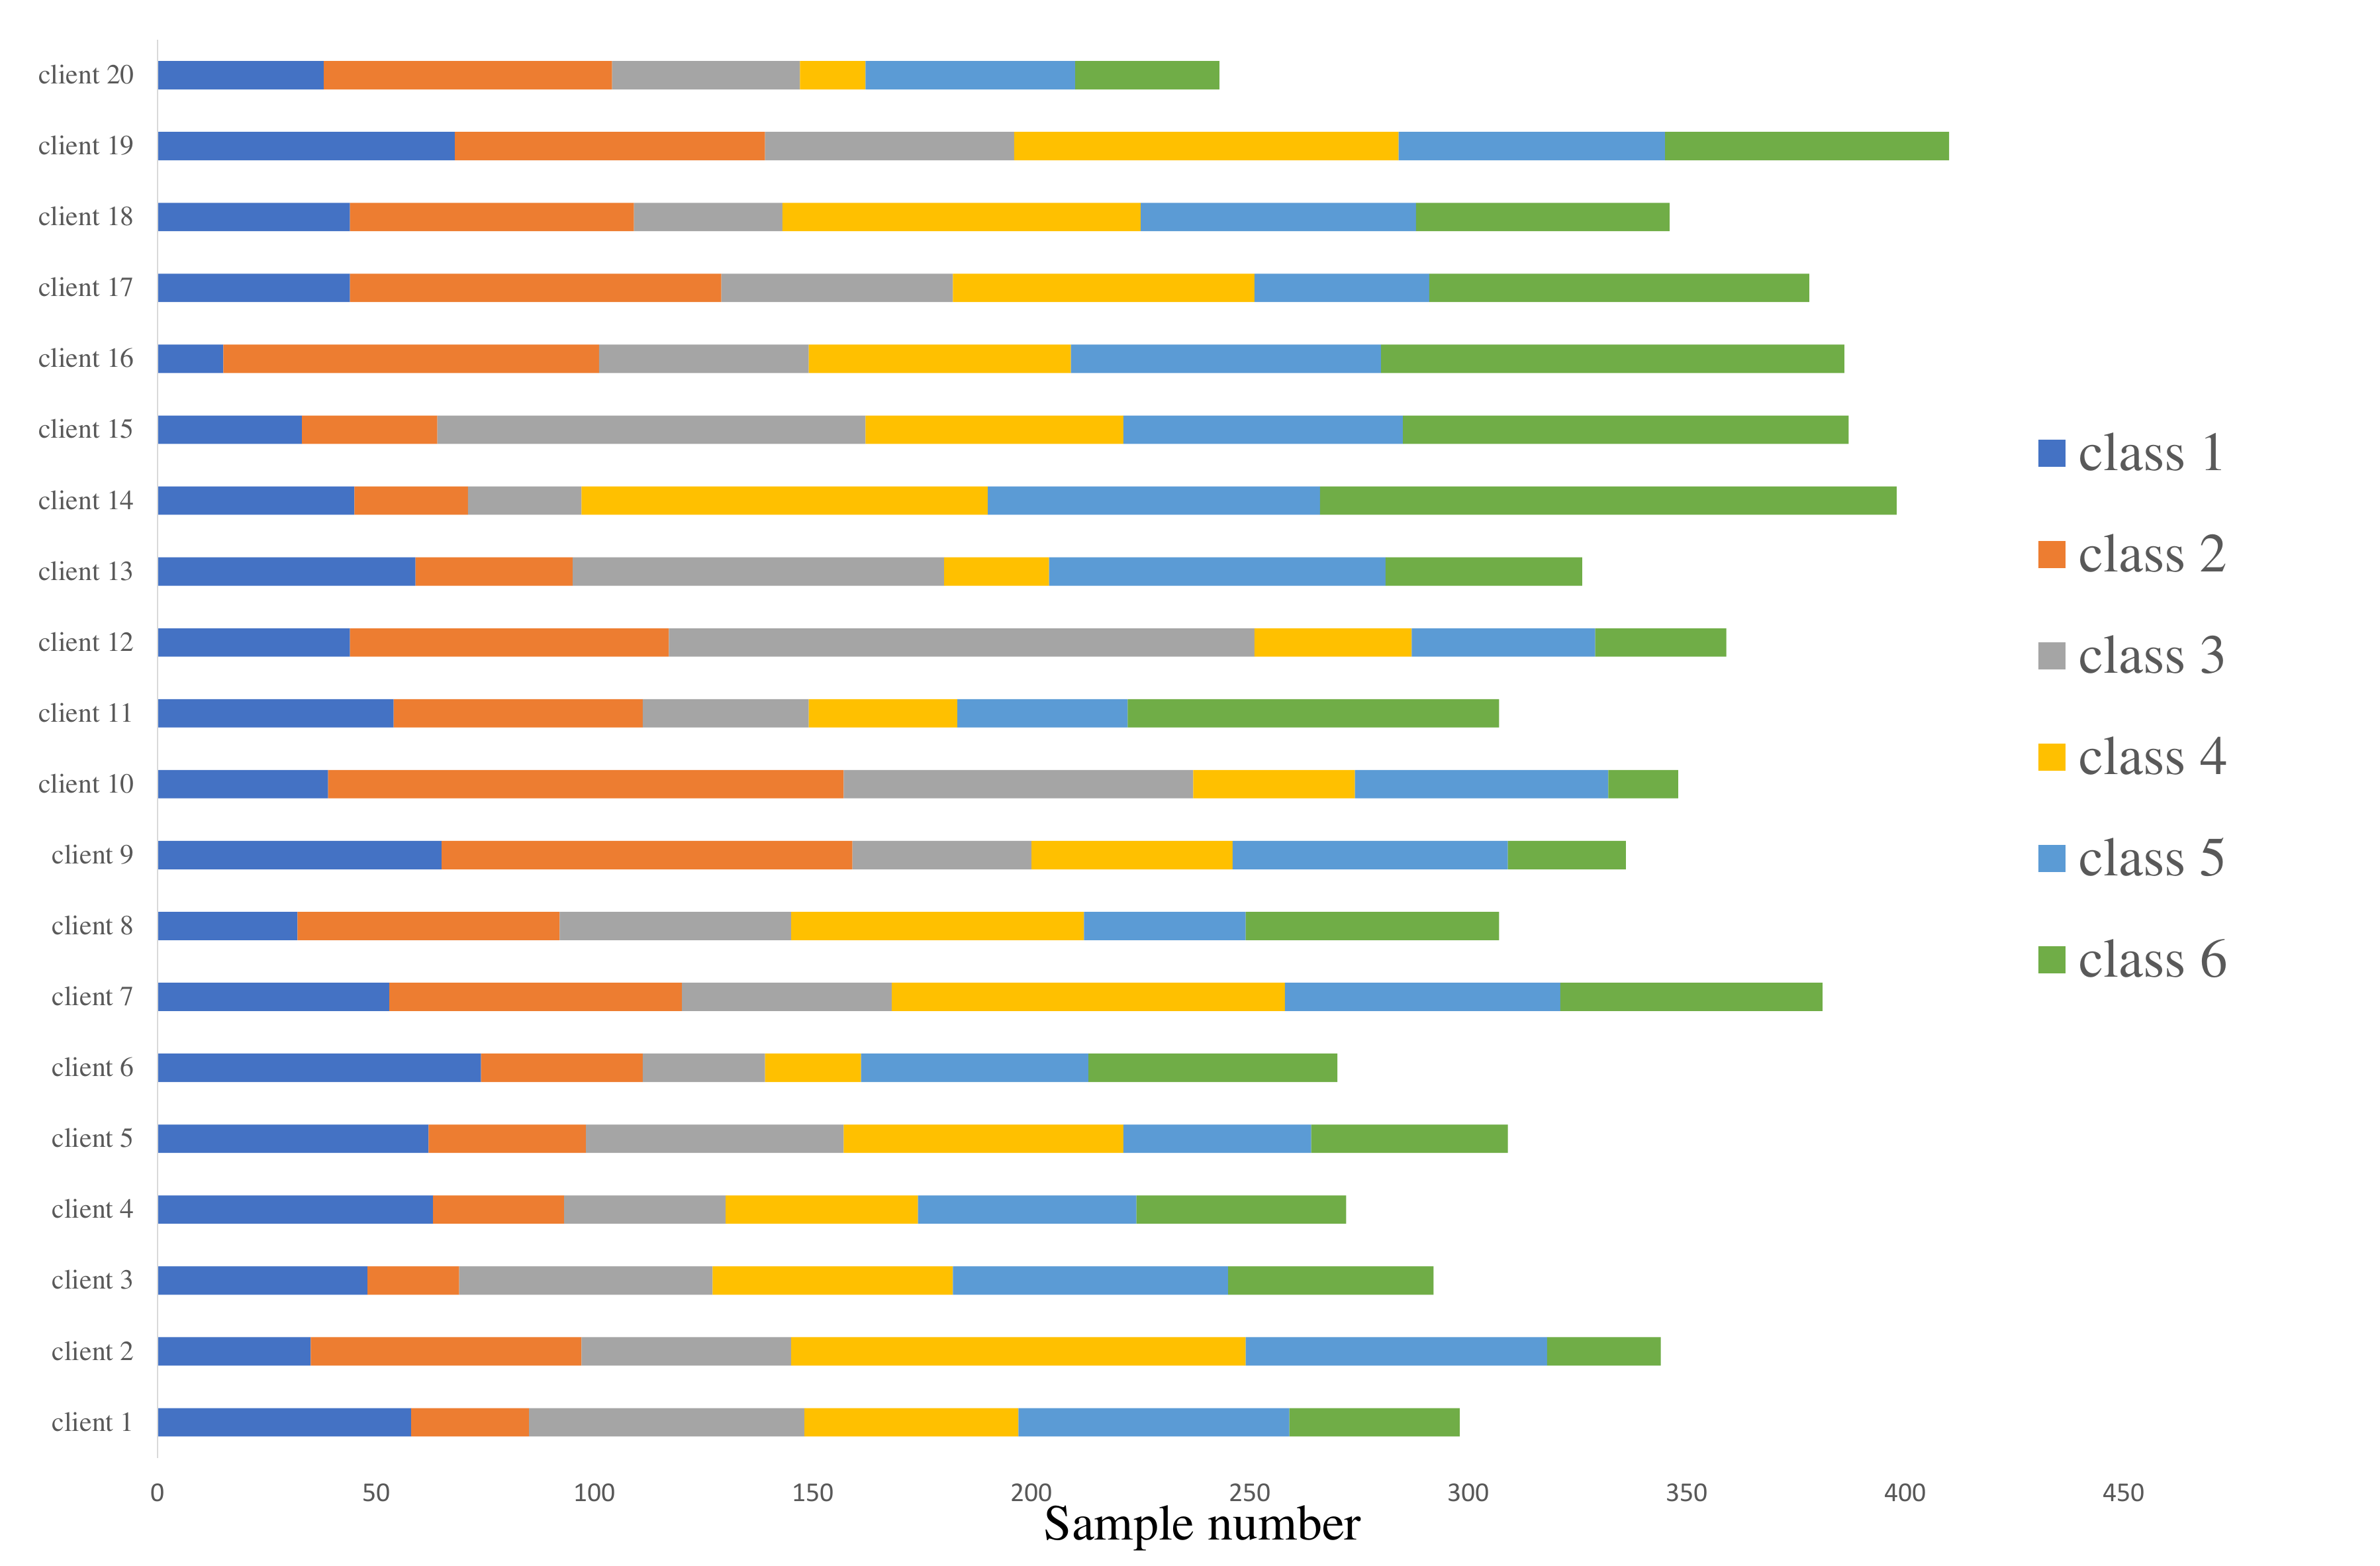}
        \caption{Non-IID}
        \label{fig:visual acc AVE}
    \end{subfigure}
    \caption{The visualization of data distribution on CREMA-D.}
    \label{fig:CREMAD client sample}
\end{figure}

\subsection{Missing Modality}
FedCMI requires knowledge transfer between modalities through local update. However there might be missing modality on some clients, making it impossible for knowledge transfer because of the lack of logit from such modality. Therefore, we only apply CMI on the clients with all modalities. The clients with missing modalities are trained with the loss $\mathcal{L} =\mathcal{L} _{ce}^{}+ \mathcal{L} _{ce}^{m}+\mathcal{L} _{prox}$

\subsection{Implementation of baselines} 
In this paper, we use seven baselines for comparison and we describe their implementation here.

For FedAvg, FedProx and FedProto, they are extended to multi-modal FL directly: perform local update based on their algorithms according to the local data and aggregation based on the sample numbers from clients. The hyper-parameter $\mu$ for FedProx is 1.0-2.0 for the three datasets according to different settings. The global prototypes for two modalities are only used in FedProto.

For FedOGM and FedPMR,  we integrate FedAvg and OGM-GE and PMR respectively. They modulate the learning paces of two modalities according to local information (without any global information).

For FedMSplit, $\gamma$ is set to 0.9 for all datasets.

\section{Experimental Results}

\noindent\textbf{The size of MLP}. In this paper, we use a two-layer MLP for both SP and IP. Here, we demonstrate the results of SP and IP with different numbers of layers. 
\begin{figure}[h]
    \centering
    \includegraphics[width=0.8\linewidth]{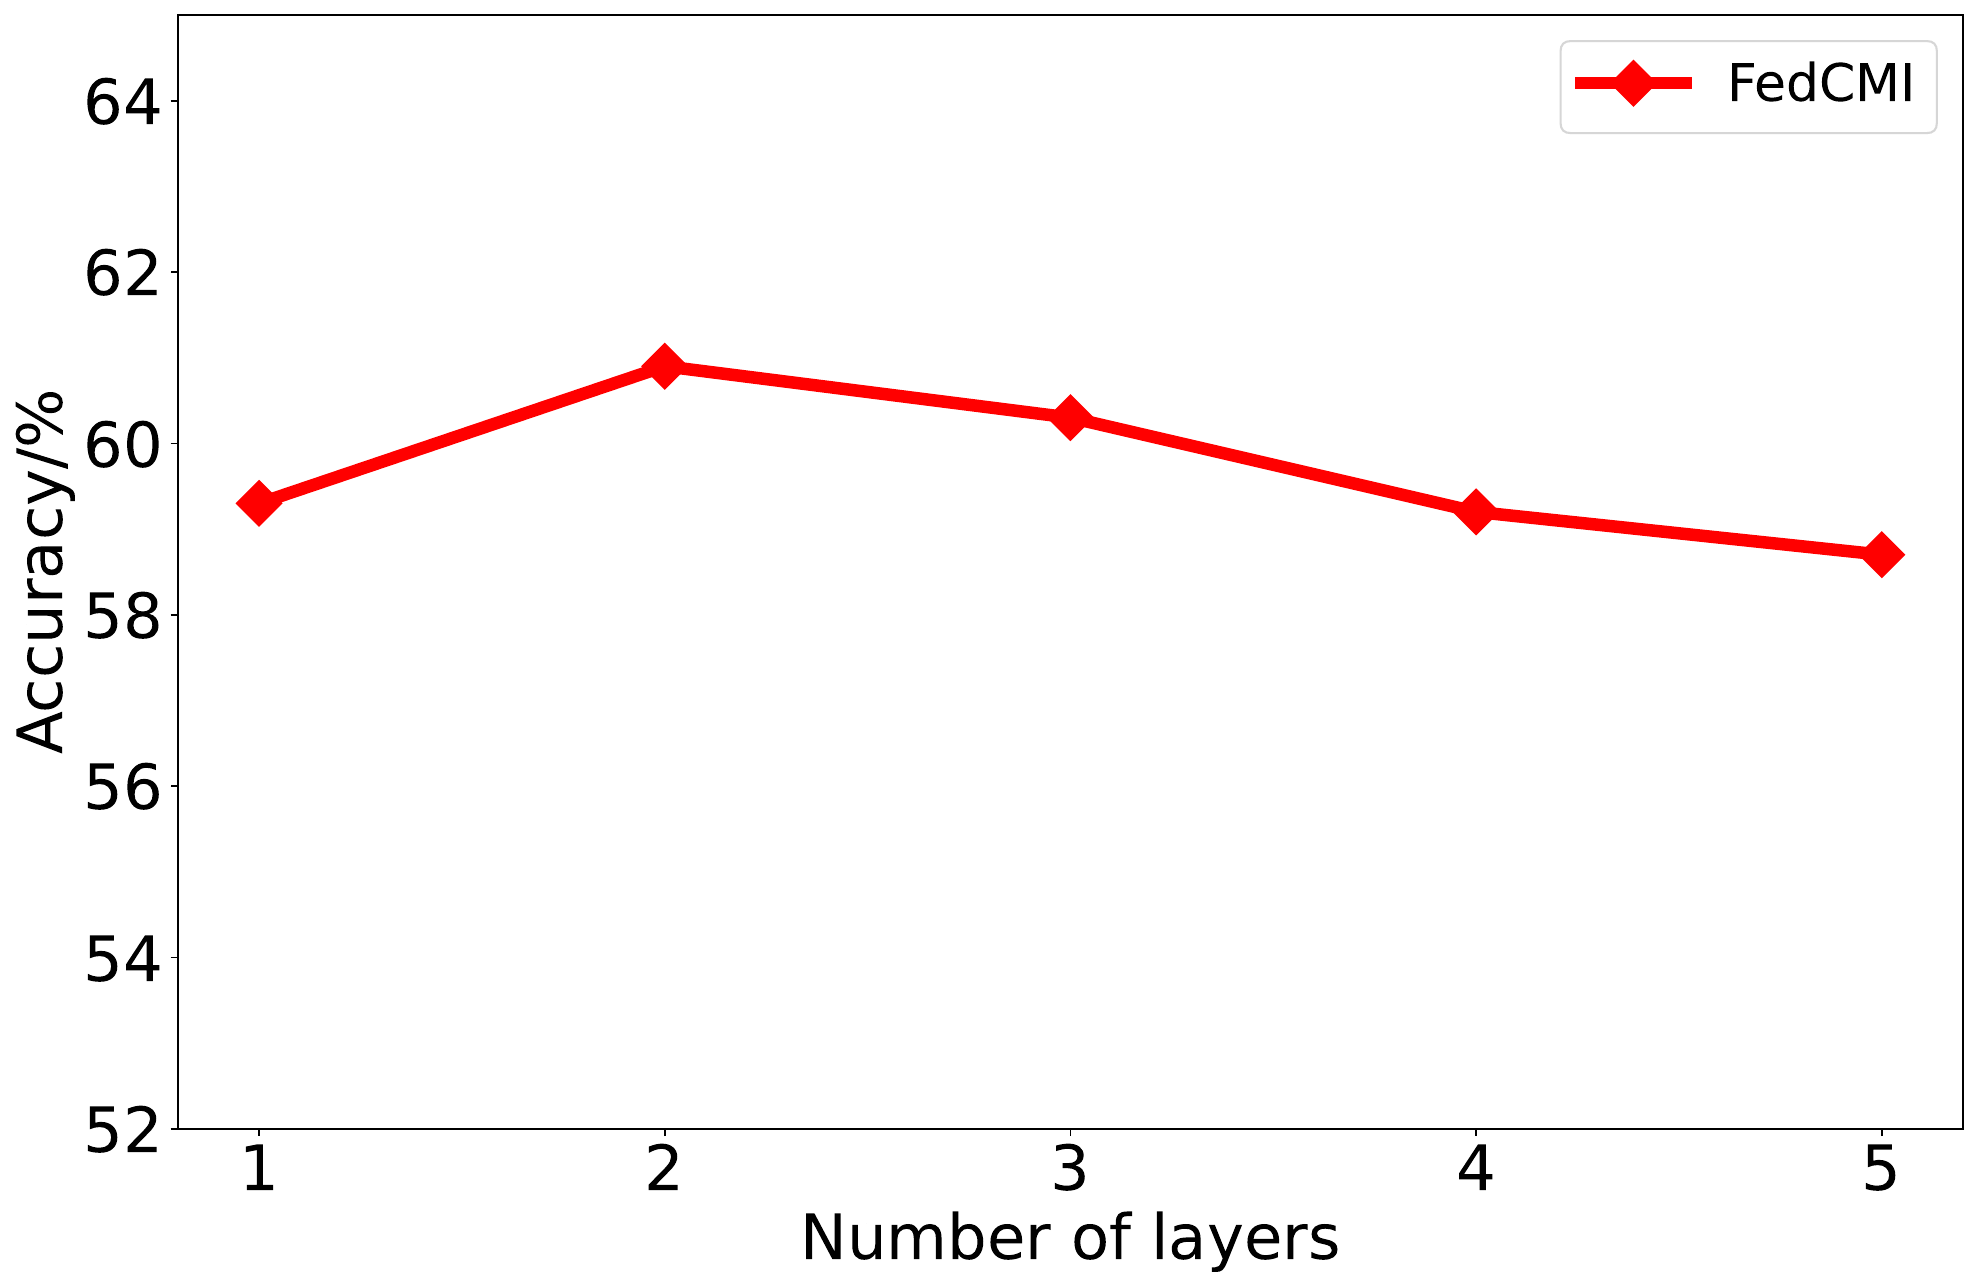}
    \caption{The performance of FedCMI with different numbers of layer for projector.}
    \label{fig: FedCMI num layer}
    % \vspace{-1.0em}
\end{figure}

It can be seen that although the difference in results using layers with different numbers is not that big, we still should choose appropriately sized projectors (SP and IP).

\noindent\textbf{More clients.}
In \cref{sec:experiment}, we use 20 clients in total for CREMA-D. To verify the effectiveness of our method on larger scale cluster, we perform experiment on CREMA-D with 50 clients under IID setting and 10 clients selected per round. The results are shown in \cref{tab:CREMA-D with 50}. It is easy to see that our FedCMI can also achieve the best performance compared with all other baselines.

\begin{table}[h]
	\centering
 % \footnotesize  
    % \caption{CIFAR-100 with VGGNet}
    \setlength{\tabcolsep}{3pt}{
	\begin{tabular}{c|c|c|c}
        \hline
        MFedAvg & MFedProx & MFedProto & FedOGM \\
        \hline
        51.1 & 51.6 & 52.2 & 56.3 \\
        \hline
        FedPMR & FedIot & FedMSplit & FedCMI \\
        \hline
        54.7 & 51.3 & 52.8 & 58.4 \\
        \hline
	\end{tabular}
 % \vspace{-1.em}
 \caption{CREMA-D with 50 clients under IID setting.}
   \label{tab:CREMA-D with 50}

 }
 % \vspace{-1.2em}
\end{table}

\textbf{}
